# Supplementary material for: Riddim: A Rhythm Analysis and Decomposition Tool Based On Independent Subspace Analysis
Source: arXiv:1705.04792 source file (2017-05-13)
Supplement: Supplementary file 1 [file appendixB.tex]

\chapter{Definitions and Mathematical Expressions}

\section{Joint Probability Distribution}

Joint Probability Distribution: 

If X and Y are discrete random variables, the function f(x,y) which
gives the probability that X = x and Y = y for each pair of values
(x,y) within the range of values of X and Y is called the joint 
probability distribution of X and Y. 

http://www.statistics.com/content/glossary/jprobdist.html

Covariance: 

The covariance between two random variables X and Y is the expected
value of the product of the variables' deviations from their means. If
there is a high probability that large values of X go with large
values of Y and small values of X go with small values of Y, then the 
covariance between X and Y will be positive; if there is a high 
probability that small values of X go with large values of Y and 
large values of X go with small values of Y, then the covariance
will be negative. 

Histogram:

A histogram is a graph of a dataset, composed of a series of
rectangles. The width of these rectangles is proportional to 
the range of values in a class or bin, all bins being the same 
width. For example, values lying between 1 and 3, between 3 and 5,
etc. The height of the rectangles is proportional to the frequency 
or the relative frequency of that class. For example the height of 
the bar centered at 2 is determined by the number of values in the 
class from 1-3.

Variance: 

Variance is a measure of dispersion. It is the average squared 
distance between the mean and each item in the population. 

Skewness:

Skewness measures the lack of symmetry of a probability distribution. 
A curve is said to be skewed to the right (or positively skewed) if 
it tails off toward the high end of the scale (right tail longer than 
the left). A curve is skewed (or negatively skewed) if it tails off 
toward the low end of the scale.
