# Supplementary material for: Riddim: A Rhythm Analysis and Decomposition Tool Based On Independent Subspace Analysis
Source: arXiv:1705.04792 source file (2017-05-13)
Supplement: Supplementary file 2 [file appendixA.tex]

\chapter{Source Code Files}

This appendix lists some examples of program code using the verbatim
environment.  If we didn't use the verbatim environment, the listing
would be interpreted as \LaTeX commands, and would not only look
bad, but also probably cause errors.

\section{ISA}
